# Supplementary material for: Gaussian Process Modelling for Improved Resolution in Faraday Depth Reconstruction
Source: arXiv:2101.07099 source file (2021-01-18)
Supplement: Supplementary file 1 [file appendix.tex]

\section{Information Criteria}
\label{app:ic}

\begin{table*}
\caption{Information criteria comparison for the \protect\cite{Sun_2015} single component Faraday thin challenge models.}
    \centering
    \begin{tabular}{@{\extracolsep{3pt}}lccccccccc@{}}
    \hline
     & \multicolumn{3}{c}{\textbf{BIC}} & \multicolumn{3}{c}{\textbf{AIC}} & \multicolumn{3}{c}{\textbf{AICc}} \\
     \cline{2-4} \cline{5-7} \cline{8-10} \\
     & HP3 & HP4 & HP5 & HP3 & HP4 & HP5 & HP3 & HP4 & HP5 \\\hline
    \textbf{Model 1} & & & & & & & & & \\
    \emph{Median} & 3755.15 & 3640.21 & 3844.46 & 3737.56 & 3618.23 & 3818.08 & 3737.50 & 3618.12 & 3817.94 \\
    \emph{IQR} & 100.50 & 60.49 & 141.18 & 100.50 & 60.49 & 141.18 & 100.50 & 60.49 & 141.18 \\
    \emph{Median Rank} & 2 & \textbf{1} & 3 & 2 & \textbf{1} & 3 & 2 & \textbf{1} & 3 \\\hline
    \textbf{Model 2} & & & & & & & & & \\
    \emph{Median} & 3470.12 & 3402.59 & 3586.46 & 3452.53 & 3380.61 & 3560.08 & 3452.46 & 3380.51 & 3559.93 \\
    \emph{IQR} & 176.85 & 140.70 & 201.36 & 176.85 & 140.70 & 201.36 & 176.85 & 140.70 & 201.36 \\
    \emph{Median Rank} & 2 & \textbf{1} & 3 & 2 & \textbf{1} & 3 & 2 & \textbf{1} & 3 \\\hline
    \textbf{Model 3} & & & & & & & & & \\
    \emph{Median} & 1747.28 & 1773.87 & 1784.08 &1729.69 & 1751.88 & 1757.70 & 1729.62 & 1751.78 & 1757.56 \\
    \emph{IQR} & 24.82 & 25.29 & 40.32 & 24.82 & 25.29 & 40.32 & 24.82 & 25.29 & 40.32 \\
    \emph{Median Rank} & \textbf{1} & 2 & 3 & \textbf{1} & 2 & 3 & \textbf{1} & 2 & 3 \\\hline
    \end{tabular}
 \label{tab:icthin}
\end{table*}

\begin{table*}
\caption{Information criteria comparison for the \protect\cite{Sun_2015} two component Faraday thin challenge models.}
    \centering
    \begin{tabular}{@{\extracolsep{3pt}}lccccccccc@{}}
    \hline
     & \multicolumn{3}{c}{\textbf{BIC}} & \multicolumn{3}{c}{\textbf{AIC}} & \multicolumn{3}{c}{\textbf{AICc}} \\
     \cline{2-4} \cline{5-7} \cline{8-10} \\
     & HP3 & HP4 & HP5 & HP3 & HP4 & HP5 & HP3 & HP4 & HP5 \\\hline
    \textbf{Model 4} & & & & & & & & & \\
    \emph{Median} & 4277.15 & 4271.52 & 4240.80 & 4259.56 & 4249.53 & 4214.42 & 4259.49 & 4249.43 & 4214.28 \\
    \emph{IQR} & 159.35 & 129.16 & 310.82 & 159.35 & 129.16 & 310.82 & 1159.35 & 129.16 & 310.82 \\
    \emph{Median Rank} & 3 & 2 & \textbf{1} & 3 & 2 & \textbf{1} & 3 & 2 & \textbf{1} \\\hline
    \textbf{Model 5} & & & & & & & & & \\
    \emph{Median} & 2243.48 & 2227.26 & 2177.76 & 2225.89 & 2205.27 & 2151.37 & 2225.82 & 2205.17 & 2151.23 \\
    \emph{IQR} & 78.90 & 47.88 & 183.96 & 78.90 & 47.88 & 183.96 & 78.90 & 47.88 & 183.96 \\
    \emph{Median Rank} & 3 & 2 & \textbf{1} & 3 & 2 & \textbf{1} & 3 & 2 & \textbf{1} \\\hline
    \textbf{Model 6} & & & & & & & & & \\
    \emph{Median} & 2607.97 & 2647.48 & 2609.77 & 2590.38 & 2625.50 & 2583.39 & 2590.31 & 2625.40 & 2583.25 \\
    \emph{IQR} & 119.54 & 242.46 & 124.85 & 119.54 & 242.46 & 124.85 & 119.54 & 242.46 & 124.85 \\
    \emph{Median Rank} & \textbf{1} & 3 & 2 & \textbf{1} & 3 & 2 & \textbf{1} & 3 & 2 \\\hline
    \textbf{Model 7} & & & & & & & & & \\
    \emph{Median} & 1938.54 & 1910.52 & 1983.06 & 1920.95 & 1888.53 & 1956.68 & 1920.88 & 1888.43 & 1956.53 \\
    \emph{IQR} & 45.77 & 113.92 & 50.01 & 45.77 & 113.92 & 50.01 & 45.77 & 113.92 & 50.01 \\
    \emph{Median Rank} & 2 & \textbf{1} & 3 & 2 & \textbf{1} & 3 & 2 & \textbf{1} & 3 \\\hline
    \textbf{Model 8} & & & & & & & & & \\
    \emph{Median} & 3752.25 & 3784.76 & 3820.70 & 3734.66 & 3762.77 & 3794.32 & 3734.59 & 3762.67 & 3794.17 \\
    \emph{IQR} & 201.42 & 259.46 & 168.60 & 201.42 & 259.46 & 168.60 & 201.42 & 259.46 & 168.60 \\
    \emph{Median Rank} & \textbf{1} & 2 & 3 & \textbf{1} & 2 & 3 & \textbf{1} & 2 & 3 \\\hline
    \textbf{Model 9} & & & & & & & & & \\
    \emph{Median} & 2480.21 & 2458.57 & 2437.71 & 2462.62 & 2436.58 & 2411.33 & 2462.55 & 2436.48 & 2411.19 \\
    \emph{IQR} & 153.57 & 154.53 & 135.08 & 153.57 & 154.53 & 135.08 & 153.57 & 154.53 & 135.08 \\
    \emph{Median Rank} & 3 & 2 & \textbf{1} & 3 & 2 & \textbf{1} & 3 & 2 & \textbf{1} \\\hline
    \textbf{Model 10} & & & & & & & & & \\
    \emph{Median} & 3715.45 & 3730.73 & 3645.83 & 3697.86 & 3708.75 & 3619.45 & 3697.80 & 3708.64 & 3619.31 \\
    \emph{IQR} & 347.43 & 262.59 & 221.87 & 347.43 & 262.59 & 221.87 & 347.43 & 262.59 & 221.87 \\
    \emph{Median Rank} & 2 & 3 & \textbf{1} & 2 & 3 & \textbf{1} & 2 & 3 & \textbf{1} \\\hline
    \textbf{Model 11} & & & & & & & & & \\
    \emph{Median} & 3644.72 & 3778.41 & 3572.76 & 3627.13 & 3756.42 & 3546.38 & 3627.06 & 3756.32 & 3546.24 \\
    \emph{IQR} & 185.38 & 122.68 & 127.99 & 185.38 & 122.68 & 127.99 & 185.38 & 122.68 & 127.99 \\
    \emph{Median Rank} & 2 & 3 & \textbf{1} & 2 & 3 & \textbf{1} & 2 & 3 & \textbf{1} \\\hline
    \textbf{Model 12} & & & & & & & & & \\
    \emph{Median} & 3645.33 & 3655.36 & 3489.09 & 3627.74 & 3633.38 & 3462.71 & 3627.67 & 3633.28 & 3462.57 \\
    \emph{IQR} & 241.72 & 315.95 & 78.99 & 241.72 & 315.95 & 78.99 & 241.72 & 315.95 & 78.99 \\
    \emph{Median Rank} & 2 & 3 & \textbf{1} & 2 & 3 & \textbf{1} & 2 & 3 & \textbf{1} \\\hline
    \textbf{Model 13} & & & & & & & & & \\
    \emph{Median} & 1843.74 & 1829.21 & 1848.77 & 1826.15 & 1807.22 & 1822.39 & 1826.08 & 1807.12 & 1822.25 \\
    \emph{IQR} & 48.46 & 31.59 & 85.03 & 48.46 & 31.59 & 85.03 & 48.46 & 31.59 & 85.03 \\
    \emph{Median Rank} & 2 & \textbf{1} & 3 & 2 & \textbf{1} & 3 & 2 & \textbf{1} & 3 \\\hline
    \end{tabular}
\label{tab:icdouble}
\end{table*}

\begin{table*}
\caption{Information criteria comparison for the \protect\cite{Sun_2015} Faraday thick challenge models.}
    \centering
    \begin{tabular}{@{\extracolsep{3pt}}lccccccccc@{}}
    \hline
     & \multicolumn{3}{c}{\textbf{BIC}} & \multicolumn{3}{c}{\textbf{AIC}} & \multicolumn{3}{c}{\textbf{AICc}} \\
     \cline{2-4} \cline{5-7} \cline{8-10} \\
     & HP3 & HP4 & HP5 & HP3 & HP4 & HP5 & HP3 & HP4 & HP5 \\\hline
    \textbf{Model 14} & & & & & & & & & \\
    \emph{Median} & 4615.45 & 4823.31 & 4834.72 & 4597.86 & 4801.32 & 4808.33 & 4597.79 & 4801.22 & 4808.19 \\
    \emph{IQR} & 246.48 & 135.32 & 144.74 & 246.48 & 135.32 & 144.74 & 246.48 & 135.32 & 144.74 \\
    \emph{Median Rank} & \textbf{1} & 2  & 3 & \textbf{1} & 2  & 3 & \textbf{1} & 2  & 3 \\\hline
    \textbf{Model 15} & & & & & & & & & \\
    \emph{Median} & 3571.76 & 3675.95 & 3755.47 & 3554.17 & 3653.97 & 3729.09 & 3554.10 & 3653.87 & 3728.95 \\
    \emph{IQR} & 216.48 & 206.81 & 297.21 & 216.48 & 206.81 & 297.21 & 216.48 & 206.81 & 297.21 \\
    \emph{Median Rank} & \textbf{1} & 2 & 3 & \textbf{1} & 2 & 3 & \textbf{1} & 2 & 3 \\\hline
    \textbf{Model 16} & & & & & & & & & \\
    \emph{Median} & 3570.51 & 3557.67 & 3468.77 & 3552.93 & 3535.69 & 3442.39 & 3552.86 & 3535.58 & 3442.25 \\
    \emph{IQR} & 213.71 & 237.92 & 223.90 & 213.71 & 237.92 & 223.90 & 213.71 & 237.92 & 223.90 \\
    \emph{Median Rank} & 3 & 2 & \textbf{1} & 3 & 2 & \textbf{1} & 3 & 2 & \textbf{1} \\\hline
    \textbf{Model 17} & & & & & & & & & \\
    \emph{Median} & 3600.12 & 3648.49 & 3698.21 & 3582.53 & 3626.51 & 3671.82 & 3582.46 & 3626.41 & 3671.68 \\
    \emph{IQR} & 102.78 & 124.75 & 138.62 & 102.78 & 124.75 & 138.62 & 102.78 & 124.75 & 138.62 \\
    \emph{Median Rank} & \textbf{1} & 2 & 3 & \textbf{1} & 2 & 3 & \textbf{1} & 2 & 3 \\\hline
    \end{tabular}
  \label{tab:icthick}
\end{table*}
